# Supplementary material for: Impact of electron solvation on ice structures at the molecular scale
Source: arXiv:1909.03844 ancillary file (2019-09-10)
Supplement: Supplementary file 1 [file supporting_information.pdf]

# Impact of electron solvation on ice structures at the molecular scale

Cord Bertram,[1,2] Philipp Auburger,[3] Michel Bockstedte,[3,4]
Julia Stähler,[5,6] Uwe Bovensiepen,[2,6] and Karina Morgenstern[1]

[1] *Physical Chemistry I, Ruhr-Universität Bochum, D-44780 Bochum, Germany*
[2] *Faculty of Physics, University of Duisburg-Essen, Lotharstr. 1, D-47057 Duisburg, Germany*
[3] *Solid State Theory, Friedrich-Alexander University Erlangen-Nürnberg, Staudtstr. 7B2, D-91058 Erlangen, Germany*
[4] *Chemistry and Physics of Materials, University of Salzburg, Jakob-Haringer-Str. 2a, A-5020 Salzburg, Austria*
[5] *Department of Physical Chemistry, Fritz Haber Institute of the Max Planck Society, Faradayweg 4-6, D-14195 Berlin, Germany*
[6] *Department of Physics, Freie Universität Berlin, Arnimallee 14, D-14195 Berlin, Germany*

## SUPPORTING INFORMATION

### STM experiments

The single-crystal Cu(111) is cleaned by repeated cycles of $Ne^+$ sputtering (1.3 keV, 1-2 $\mu$A, 45 min) and annealing at 900 K for 20 min and for 10 min in the last cycle. During all procedures applied to the sample the pressure is below $4.0 \cdot 10^{-10}$ mbar.

$D_2O$ is filled into a glass tube, which is attached to a separately pumped chamber. It is degassed under vacuum to remove remaining impurities by several freeze-pump-thaw cycles through a line that does not pass the main chamber. $D_2O$ has a sufficiently high vapor pressure at room temperature for deposition. The vapor is introduced into the main chamber through a leak valve, which opens into a stainless steel tube that points towards the sample. Every hot filament is switched off during deposition in order to suppress dissociation of the molecules.

| $\lambda$ (nm) | h$\nu$ (eV) | $P$ ($\mu$W) | $\alpha$ | $F$ (pJ/cm$^2$) |
|---|---|---|---|---|
| 330 | 3.77 | 0.23 | 0.63 | 7.0 |
| 340 | 3.65 | 0.44 | 0.62 | 13.1 |
| 350 | 3.55 | 0.69 | 0.61 | 20.2 |
| 360 | 3.44 | 0.83 | 0.59 | 23.9 |
| 370 | 3.36 | 0.83 | 0.58 | 23.5 |
| 380 | 3.27 | 0.89 | 0.57 | 24.8 |
| 390 | 3.19 | 1.11 | 0.57 | 30.4 |
| 400 | 3.11 | 1.33 | 0.56 | 35.8 |
| 410 | 3.03 | 1.37 | 0.55 | 36.2 |
| 420 | 2.95 | 1.22 | 0.54 | 35.6 |
| 430 | 2.89 | 1.03 | 0.54 | 31.2 |
| 440 | 2.82 | 1.10 | 0.53 | 26.0 |
| 450 | 2.75 | 1.29 | 0.52 | 27.4 |

Table I. Dependence of measured power $P$ and calculated laser fluence $F$ in Cu(111) behind an aperture (size: 0.026 mm$^2$) on wavelength $\lambda$, photon energy h$\nu$, absorbance $\alpha$ for incident angle of 79° (parameters from [1]).

The illumination experiments were performed with a frequency-doubled super-continuum laser including a Extend-UV light source supplied by a SuperK Extreme pump laser from NKT Photonics. The laser has a repetition rate of 77.8 MHz and a pulse length of around 10 ps. The laser beam enters the tip surface region via a lens system through a UV-transmitting sapphire window into the UHV chamber and through closable holes in the cryo shields that surround the STM. The beam is focused underneath the tip with the aid of external mirrors. At close to grazing incident angle, the spot is elliptical with wave length dependent diameters (2.05 mm to 1.54 mm; 0.41 mm to 0.95 mm) on Cu(111). The spot of the laser is thus always much larger than the area imaged by STM. We determine the absorbed fluence $F$ in the tip region in a separate setup by transmission through a pinhole with an radius of 40 $\mu$m. This separate setup mimics the path of the laser to the sample and the angle of 79° with respect to the surface normal. The calculation considers the wavelength dependent absorbance factor $\alpha$ from literature [1]. Photon doses per molecule are determined from the absorbed fluences; for crystalline ice based on its previously determined structure and for the 40% less dense amorphous ice corrected by a factor of 2.5 [2].

During illumination, the surface temperature rises continuously from the measurement temperature of 7.5 K to a temperature of 10.3 K at most. In order to exclude that thermal effects and effects due to tip-sample interaction are at the origin of the observed changes, the system is heated to 12 K without illumination and scanned in the same manner as during the illumination experiments. The differences between changes observed with and without illumination are at least one order of magnitude.

The dissociation of water molecules is indicated by a contrast inversion in STM [10]. Since the molecules do not change their appearance during illumination, they thus remain intact while irradiated with UV light.

The cross section $\sigma$ describes the structural rearrangements measured by STM. It represents the probability to induce a local, molecular change in structure taking the available photons and water molecules into account. In

detail, we determine $\sigma$ as

$$\sigma = \frac{N_E}{A_{island}} \cdot \frac{1}{\rho_{ph} \cdot \rho_{D2O}} \quad (1)$$

Since the adsorbed water forms islands at the investigated coverage, the area $A_{island}$ represents the fraction of the surface area, which is covered by ice. Only in this region, water molecules may rearrange. The number of rearranged water molecules is $N_E$. The ratio $N_E/A_{island}$ thus corresponds to the density of local permanent rearrangements. It is normalized to the density of absorbed photons during illumination $\rho_{ph}$ and the density of water molecules per surface area $\rho_{D2O}$. For our ice structures, $A_{island}$=215…1519 nm$^2$, $N_E$=19…73, $\rho_{D2O}$=11.36 nm$^{-2}$ [2], and $\rho_{ph}$=0.2…1.2·10$^{20}$ photons/cm$^2$ depending on photon energy. The cross section $\sigma$ as determined directly from the STM experiment ranges thus from 0.2 to 1.0·10$^{-22}$ cm$^2$ (see Fig. 4c). This finding corresponds to $\sigma \cdot \rho_{D2O}$=0.3…1.1·10$^{-7}$ rearrangements per incident photon.

To exploit the connection to electron solvation, we estimate the probability of a photon to inject an electron into the ice. Only the electrons excited within approximately the first nanometer of Cu can reach the metal-ice interface and thus be transferred to the ice and get solvated. Only 7% of the photons are absorbed within the first nm according to the copper refractive index at the angle of incidence of 45°. Half of these electrons have a positive momentum component along the surface normal. Only those electrons that have energies beyond 3.1 eV can get transferred into the ice [3]. This fraction increases with increasing photon energy. It is estimated here to reduce the number of transferred electrons by around one order of magnitude. This estimation suggests that there are around $10^{-2}$ injected electrons per incident photon. Note, that in this rough estimate, we disregard the reflection of electrons at the ice-metal interface.

According to these two estimates, the probability for an injected electron to induce a molecular rearrangement is $10^{-5}$. This is a typical value for electron induced molecular rearrangements in inelastic electron tunneling experiments (Chapter 7 in [4], cf. [5, 6]).

## 2PPE experiments

Very similar to the STM preparation, the single-crystal Cu(111) is cleaned by repeated cycles of $Ar^+$ sputtering (0.7 keV, 1.5 $\mu$A, 5 min) and annealing at 700 K for 20 min. The surface quality was checked by low-energy electron diffraction (LEED), work function measurements, and the width of the Shockley surface state in photoemission spectra. $D_2O$ is filled into a glass tube, which is attached to a separately pumped gas system, in which several freeze-pump-thaw cycles were performed for purification. The $D_2O$ vapor is introduced into the main chamber through a pinhole doser in line of sight of the sample surface. Photoemission experiments are performed at a sample temperature of 30 K using a regeneratively amplified femtosecond laser system described in detail elsewhere [11]. It drives an optical parametric amplifier providing $h\nu_{\mathrm{probe}} = 2.04$ eV laser pulses at a repetition rate of 200 kHz. These are frequency doubled in a BBO crystal to generate UV laser pulses at $h\nu_{\mathrm{pump}} = 3.99$ eV. The cross correlation of the pump and probe laser pulses is measured directly at the sample and yields 40 fs average laser pulse duration. The UV laser pulses are used to photoexcite the sample and $h\nu_{\mathrm{probe}}$ for photoemission of the transient electron population in normally unoccupied states. We measure the kinetic energy of the photoelectrons using an electron time-of-flight spectrometer with an energy resolution < 20 meV. The spectra are plotted versus the intermediate state energy with respect to the Fermi level: $E - E_{\mathrm{F}} = E_{\mathrm{kin}} + \Phi - h\nu_{\mathrm{probe}}$, with the sample work function $\Phi = E_{\mathrm{vac}} - E_{\mathrm{F}}$.

## Ab initio modeling

For calculations, a slab model consisting of three bilayers in a $(2 \times 6)$ unit cell represents the hexagonal ice surface. On top of this slab, admolecule structures are assembled. Together with a vacuum region of 2.17 nm between the surfaces, this yields well converged electronic properties. Protons within the bilayer are arranged in a fashion to cancel the total dipole moment. This antiferroelectric proton order between two bilayers reduces the complexity of the calculations. On top of the slab, several proton arrangements within each admolecule structure are tested to identify arrangements with low energy and large electron affinity. Electronic wave functions are represented by a projector augmented plane-wave basis set (PAW) as implemented for all levels of theory in the VASP-package (for details cf. [7, 8] and references therein). Plane waves up to a cut-off energy of 400 eV are included. This basis set yields well-converged properties at all levels of theory as extensive tests show. All structures are fully relaxed until forces are lower than 0.03 eV/nm. Here, semi-empirical dispersion corrections are not employed as discussed in [9]. GW calculations are performed based on the wave functions obtained at the PBE0-level of theory including virtual states in an energy range up to 125 eV. This provides a more consistent starting point than the PBE-level for the trapped excess electron due to its superior cancellation of the self-interaction. For the ice surface, the results are compared with self-consistent GW0 calculations: The inclusion of self-consistency yields only minor corrections for the position of the ice conduction bands. This observation is expected to hold for excess electron states which extend

over a few water molecules.

[1] K. Stahrenberg, Th. Herrmann, K. Wilmers, N. Esser, W. Richter, M. J. G. Lee, Phys. Rev. B **64**, 115111 (2001).
[2] M. Mehlhorn, K. Morgenstern, Phys. Rev. Lett. **99**, 246101 (2007).
[3] J. Sthler, J.-C. Deinert, D. Wegkamp, S. Hagen, M. Wolf, J. Am. Chem. Soc. **137**, 3520-3524 (2015).
[4] K. Morgenstern, N. Lorente, K.-H. Rieder, Phys. Status Solidi B, 1-81 (2013).
[5] M. Mehlhorn, J. Carrasco, A. Michaelides, K. Morgenstern, Phys. Rev. Lett. 101, 026101 (2009).
[6] H. Gawronski, J. Carrasco, A. Michaelides, K. Morgenstern, Phys. Rev. Lett. **101**, 136102 (2008).
[7] G. Kresse, D. Joubert, Phys. Rev. B **59**, 1758 (1999).
[8] M. Shishkin, G. Kresse, Phys. Rev. B **75**, 235102 (2007).
[9] M. Bockstedte, A. Michl, M. Kolb, M. Mehlhorn, K. Morgenstern, J. Phys. Chem. C **120**, 1097-1109 (2016).
[10] M. Mehlhorn, H. Gawronski, K. Morgenstern, Phys. Rev. Lett. **101**, 196101 (2008).
[11] M. Lisowski, P. A. Loukakos, U. Bovensiepen, J. Sthler, C. Gahl, M. Wolf, Appl. Phys. A **78**, 165 (2004).
